# Supplementary material for: Low-bit Model Quantization for Deep Neural Networks: A Survey
Source: arXiv:2505.05530 source file (2025-05-08)
Supplement: Supplementary file 1 [file supp.pdf]

# Supplementary File: Low-bit Model Quantization for Deep Neural Networks: A Survey

Kai Liu†, Qian Zheng†, Kaiwen Tao†, Zhiteng Li, Haotong Qin, Wenbo Li, Yong Guo, Xianglong Liu, Linghe Kong∗, Guihai Chen, *Fellow, IEEE*, Yulun Zhang∗, Xiaokang Yang, *Fellow, IEEE*

## 1 Common Information of Quantization

Different tasks, such as image classification, image generation, and text understanding, usually need different quantization methods due to the varying characteristics of weights and activation. Here, we collect the frequently studied 7 tasks in the field of quantization, including text-to-text (T2T), image-to-text (I2T), visual generation, super-resolution, image segmentation, image classification, and object detection. Also, we collect the commonly used datasets and models in these tasks, and representative papers, as shown in Tab 1. We tried to provide the performance comparison of different quantization methods on these benchmarks, but failed. This is because the models, datasets, and quantification schemes adopted by the recent methods are all different, leading to an exponential number of experiments. We hope that Tab 1 can help the emerging forces in the model quantization quickly understand the cutting edge of quantization methods and thereby promote the development.

## 2 Related Works

Many works also investigate the model compression techniques [89]–[96].

Rokh *et al.* [90] provides a comprehensive overview of model quantization techniques for deep neural networks (DNNs) in the context of image classification. The authors delve into the fundamental concepts of quantization, exploring various methods and approaches that have been proposed to reduce the memory footprint and computational complexity of DNNs while maintaining their accuracy. The survey categorizes and discusses different quantization strategies, including clustering-based methods, uniform and non-uniform quantization, and the use of scale factors to enhance quantization accuracy. Additionally, it examines the training of quantized neural networks, highlighting the role of techniques such as the straight-through estimator and quantization regularization. The sensitivity of different layers to quantization is analyzed, and the performance of state-of-the-art methods on benchmark datasets like CIFAR-10 and ImageNet is presented. However, it fails to cover quantization methods in other areas, such as large language models and other computer vision tasks. On the contrary, we provide a more comprehensive and updated view of model quantization.

Gholami *et al.* [91] provides a comprehensive overview of quantization methods aimed at enhancing the efficiency of neural network inference. It delves into the fundamental concepts and advanced techniques employed in quantizing neural networks, highlighting the trade-offs between precision, accuracy, and computational efficiency. The authors categorize various quantization approaches, including uniform and non-uniform quantization, symmetric and asymmetric schemes, and different calibration methods. They also discuss the impact of quantization granularity, ranging from layer-wise to channel-wise quantization, and the implications for hardware deployment. The survey further explores the integration of quantization with other optimization techniques such as knowledge distillation and pruning, emphasizing the potential for mixed-precision quantization to balance accuracy and efficiency. Additionally, it examines the challenges and opportunities in hardware-aware quantization, particularly for edge devices.

The survey by Shen *et al.* [95] provides a comprehensive exploration of quantization techniques for LLMs, categorizing them into three primary approaches: post-training quantization, quantization-aware fine-tuning, and quantization-aware training. PTQ methods, which apply quantization after pre-training, offer simplicity and efficiency but may introduce performance degradation. QAF techniques integrate quantization during the fine-tuning phase to compensate for some of the quantization losses, achieving a balance between accuracy and computational efficiency. QAT, which incorporates quantization directly into the training process, enables models to adapt to low-precision representations


- † *denotes equal contribution.*
- *Kai Liu, Qian Zheng, Kaiwen Tao, Zhiteng Li, Linghe Kong, Guihai Chen, Yulun Zhang, and Xiaokang Yang are with the School of Computer Science, Shanghai Jiao Tong University, Shanghai, China. Email: normal.kliu@gmail.com, xiaozheng2023@sjtu.edu.cn, miukiii19@sjtu.edu.cn, ieeezhitengli@gmail.com, linghe.kong@sjtu.edu.cn, gchen@cs.sjtu.edu.cn, yulun100@gmail.com, xkyang@sjtu.edu.cn.*
- *Haotong Qin is with ETH Zürich, Switzerland. (Email: qinhaotong@gmail.com).*
- *Wenbo Li is with Huawei Noah's Ark Lab, China. (Email: wenboli@cse.cuhk.edu.hk). Yong Guo is with Huawei Consumer Business Group, China. (E-mail: guoyongcs@gmail.com).*
- *Xianglong Liu is with Beihang University, China. (Email: xlliu@buaa.edu.cn).*
- *Yulun Zhang and Linghe Kong are the corresponding authors.*


0000–0000/00$00.00 © 2021 IEEE

TABLE 1
Common Datasets, Models, and Representative Papers for Various Tasks

| Tasks | Training Dataset | Testing Dataset | Models | Representative Papers |
|---|---|---|---|---|
| T2T | Wikitext [1], WikiText2 [1], C4 [2], HH-RLHF [3], Alpaca [4], Flan v2 [5], SQuAD1.1 [6] | Wikitext [1], C4 [2], WikiText2 [1], PTB [7], GLUE [8], Super-NaturalInstructions [9], PIQA [10], ARC-e, ARC-c, HellaSwag [11], Winogrande [12], | Transformer [13], OPT [14], Bloom [15], GLM [16], MT-NLG [17], Llama-2 [18], Falcon [19], Mixral [20], BERT [21], RoBERTa [22], XLNet [23], GPT-3 [24], GPT-4 [25], T5 [2], Mistral [26], Starcoder [27], Gemma [28], [29] | ZeroQuant [30], Smoothquant [31], Squeezellm [32], Q-BERT [33], Qlora [34], GPTQ [35], SpQR [36], AWQ [37], [38] |
| I2T | Obelics [39], LAION-5B [40], Wikipedia-based Image Text [41] | GQA [42], TextVQA [43], ScienceQA [44], VizWiz [45] | VICUNA-V1.5 [], LLAVA-V1.5 [46], MoE-LLaVA, OpenFlamingo [47] | [48] |
| Visual Generation | ImageNet [49], CIFAR-10 [50], LSUN, COCO [51] | ImageNet [49], CIFAR-10 [50], LSUN-Bedrooms [52], LSUN-Churches [52], COCO [51], SQuAD1.1 [6], VQA-v2 [53], GQA [42], VizWiz [45], SQAI [44], VQAT [43] | DDIM [54], DDPM [55], ResNet [56], MobileNetV2 [57], Swin , BERT [21], RoBERTa [22], LLaVA [46], FFHQ [58], VILA [59], transformer [60] | AWQ [37] QDROP [61], PTQ4DM [62], [63], [64], |
| Super Resolution | DIV2K [65], DRealSR [66], | Set5 [67], Set14 [68], B100 [69], Urban100 [70], DRealSR [66] | VDSR [71], EDSR [72], RDN [73], SRResNet [74] | DAQ [75] SLB [76], [77], |
| Image Segmentation | COCO [51], ImageNet [49] | ImageNet [49] | Enet, DeepLabV3+ [78], RepVGG [79] | AdaRound [80] |
| Image Classification | ImageNet [49], CIFAR-10 [50], ILSVRC2012 | ImageNet [49], CIFAR-10 [50], ILSVRC2012 | Enet, ResNet [56], MobileNetV2 [57], RegNet [81], MnasNet [82], RepVGG [79], VGG-Small [83], Inception-V3 [84] | QDROP [61], BRECQ [85], HAWQ [86], [87] |
| Object Detection | COCO [51] | COCO [51] | One-stage RetinaNet [88], ResNet [56], Enet, RepVGG [79] | QDROP [61], BRECQ [85] |

from the outset, potentially yielding more robust and efficient quantized models. The survey also highlights experimental studies that uncover underlying patterns and challenges in LLM quantization, providing valuable insights for future research. However, this survey only investigates a limited papers and only focuses on LLM instead of other advanced models.

As LLMs become crucial, some works thoroughly evaluate quantization methods on LLMs [92], [94], [96]. Li *et al.* [92] present a thorough evaluation of efficiency and performance by evaluating the effect of PTQ on weight, activation, and KV Cache on 11 model families. While Dettmers *et al.* [96] study the trade-off between the size of the base model and bit-width by developing inference scaling laws of zero-shot performance in LLMs to determine the bit-precision and model size that maximize performance. Yao *et al.* [94] conduct a comprehensive experiments of diverse PTQ on weight-only, activation-only, and weight-and-activation quantization.

## 3 Other Model Compression Techniques

**a) Pruning:** Pruning aims to remove redundant structures to compress DNNs. Redundancies is identified based on different criteria such as sparsity [97]–[99], Bayesian pruning [100], [101], importance ranking [102], [103], grouped kernel search [104], reinforcement learning [105], and the lottery ticket hypothesis [106]. Pruning strategies are broadly classified into two categories: structured and unstructured. Structured pruning [107], [108] involves the removal of entire neurons or filters, while unstructured pruning [109] operates at the weight level by removing individual weights or neurons based on their importance. Structure pruning enjoys better alignment with existing hardware and software acceleration frameworks, but suffers from bigger performance degradation. As for unstructured pruning, finer granularity allows a sparser model and higher precision in preserving model performance.

**b) Knowledge Distillation:** Knowledge distillation [110]–[113], also known as model distillation, is a technique for transferring knowledge from the teacher model to the student model, while the former is large and complex and the latter is small and simple. The core idea behind this method is that a well-trained teacher model encodes explicit knowledge in its weights and also implicitly captures deep-level features and patterns in its internal representations, which can be passed on to the student model through specific technical means. In the current context, knowledge distillation has been developed into many variants, and one-step distillation for diffusion models is increasingly popular.

**c) Model Design:** Lightweight network design focuses on optimizing the model architecture to reduce the number of parameters. In recent years, various lightweight network

architectures [60], [114], [115] have been proposed. These architectures incorporate modern designs, such as attention mechanisms and Mamba architecture, to reduce model complexity while maintaining high performance.

## 4 Why Quantization Brings Acceleration

The acceleration of quantization is mainly attributed to the following reasons:

*Memory Access Acceleration.* Quantization alleviates memory bottlenecks through precision reduction, compressing weight and activation representations. Since modern computing chips often suffer from memory bottlenecks where computational power far exceeds memory throughput, quantization directly reduces the memory footprint and the volume of data transfer. Additionally, theoretical analysis has consistently demonstrated that memory access optimization often dominates overall speedup despite computational overhead from weight dequantization.

*Vectorization.* Efficient vectorized computing instructions are fundamentally engineered to exploit data-level parallelism in large-scale computational workloads. For example, a 512-bit register natively processes 16 operands of FP32. With INT8 quantization, equivalent hardware resources enable 64-element parallel execution. Moreover, integer operations often take less time and energy than floating-point operations. Compiler-assisted optimizations further maximize hardware utilization through instruction scheduling and memory access pattern alignment.

Researchers also focus on the overhead brought by the quantization and dequantization processes. Techniques like operator fusion and computation graph optimization are investigated to minimize or eliminate the overhead.

## References


[1] S. Merity, C. Xiong, J. Bradbury, and R. Socher, "Pointer sentinel mixture models," in *Proc. Int. Conf. Learn. Represent.*, 2017.

[2] C. Raffel, N. Shazeer, A. Roberts, K. Lee, S. Narang, M. Matena, Y. Zhou, W. Li, and P. J. Liu, "Exploring the limits of transfer learning with a unified text-to-text transformer," *Journal of machine learning research*, vol. 21, no. 140, pp. 1–67, 2020.

[3] Y. Bai, A. Jones, K. Ndousse, A. Askell, A. Chen, N. DasSarma, D. Drain, S. Fort, D. Ganguli, T. Henighan *et al.*, "Training a helpful and harmless assistant with reinforcement learning from human feedback," *arXiv preprint arXiv:2204.05862*, 2022.

[4] R. Taori, I. Gulrajani, T. Zhang, Y. Dubois, X. Li, C. Guestrin, P. Liang, and T. B. Hashimoto, "Stanford alpaca: An instruction-following llama model," 2023.

[5] S. Longpre, L. Hou, T. Vu, A. Webson, H. W. Chung, Y. Tay, D. Zhou, Q. V. Le, B. Zoph, J. Wei *et al.*, "The flan collection: Designing data and methods for effective instruction tuning," in *Proc. Int. Conf. Mach. Learn.* PMLR, 2023, pp. 22 631–22 648.

[6] P. Rajpurkar, J. Zhang, K. Lopyrev, and P. Liang, "Squad: 100,000+ questions for machine comprehension of text," in *Proc. Conf. Empir. Methods Nat. Lang. Process.*, 2016.

[7] M. Marcus, G. Kim, M. A. Marcinkiewicz, R. MacIntyre, A. Bies, M. Ferguson, K. Katz, and B. Schasberger, "The penn treebank: annotating predicate argument structure," in *Proceedings of the Workshop on Human Language Technology*, 1994, p. 114–119.

[8] A. Wang, A. Singh, J. Michael, F. Hill, O. Levy, and S. R. Bowman, "Glue: A multi-task benchmark and analysis platform for natural language understanding," in *Proc. Int. Conf. Learn. Represent.*, 2019.

[9] Y. Wang, S. Mishra, P. Alipoormolabashi, Y. Kordi, A. Mirzaei, A. Arunkumar, A. Ashok, A. S. Dhanasekaran, A. Naik, D. Stap *et al.*, "Super-naturalinstructions: Generalization via declarative instructions on 1600+ nlp tasks," in *Proc. Conf. Empir. Methods Nat. Lang. Process.*, 2022.

[10] Y. Bisk, R. Zellers, R. L. Bras, J. Gao, and Y. Choi, "Piqa: Reasoning about physical commonsense in natural language," in *Proc. AAAI Conf. Artif. Intell.*, 2020.

[11] R. Zellers, A. Holtzman, Y. Bisk, A. Farhadi, and Y. Choi, "Hellaswag: Can a machine really finish your sentence?" in *Proc. Annu. Meeting Assoc. Comput. Linguistics*, 2019.

[12] K. Sakaguchi, R. L. Bras, C. Bhagavatula, and Y. Choi, "Winogrande: An adversarial winograd schema challenge at scale," *CoRR*, 2019.

[13] A. Vaswani, N. Shazeer, N. Parmar, J. Uszkoreit, L. Jones, A. N. Gomez, Ł. Kaiser, and I. Polosukhin, "Attention is all you need," in *Proc. Adv. Neural Inform. Process. Syst.*, vol. 30, 2017.

[14] S. Zhang, S. Roller, N. Goyal, M. Artetxe, M. Chen, S. Chen, C. Dewan, M. Diab, X. Li, X. V. Lin *et al.*, "Opt: Open pre-trained transformer language models," *arXiv preprint arXiv:2205.01068*, 2022.

[15] B. Workshop, T. L. Scao, A. Fan, C. Akiki, E. Pavlick, S. Ilić, D. Hesslow, R. Castagné, A. S. Luccioni, F. Yvon *et al.*, "Bloom: A 176b-parameter open-access multilingual language model," *arXiv preprint arXiv:2211.05100*, 2022.

[16] A. Zeng, X. Liu, Z. Du, Z. Wang, H. Lai, M. Ding, Z. Yang, Y. Xu, W. Zheng, X. Xia *et al.*, "Glm-130b: An open bilingual pre-trained model," in *Proc. Int. Conf. Learn. Represent.*, 2023.

[17] S. Smith, M. Patwary, B. Norick, P. LeGresley, S. Rajbhandari, J. Casper, Z. Liu, S. Prabhumoye, G. Zerveas, V. Korthikanti *et al.*, "Using deepspeed and megatron to train megatron-turing nlg 530b, a large-scale generative language model," *arXiv preprint arXiv:2201.11990*, 2022.

[18] H. Touvron, L. Martin, K. Stone, P. Albert, A. Almahairi, Y. Babaei, N. Bashlykov, S. Batra, P. Bhargava, S. Bhosale *et al.*, "Llama 2: Open foundation and fine-tuned chat models," *arXiv preprint arXiv:2307.09288*, 2023.

[19] E. Almazrouei, H. Alobeidli, A. Alshamsi, A. Cappelli, R. Cojocaru, M. Debbah, É. Goffinet, D. Hesslow, J. Launay, Q. Malartic *et al.*, "The falcon series of open language models," *arXiv preprint arXiv:2311.16867*, 2023.

[20] A. Q. Jiang, A. Sablayrolles, A. Roux, A. Mensch, B. Savary, C. Bamford, D. S. Chaplot, D. d. l. Casas, E. B. Hanna, F. Bressand *et al.*, "Mixtral of experts," *arXiv preprint arXiv:2401.04088*, 2024.

[21] J. Devlin, M.-W. Chang, K. Lee, and K. Toutanova, "Bert: Pre-training of deep bidirectional transformers for language understanding," in *Proc. 2019 NAACL - HLT, Vol. 1 (Long & Short Papers)*, 2019, pp. 4171–4186.

[22] Y. Liu, M. Ott, N. Goyal, J. Du, M. Joshi, D. Chen, O. Levy, M. Lewis, L. Zettlemoyer, and V. Stoyanov, "Roberta: A robustly optimized bert pretraining approach," *arXiv preprint arXiv:1907.11692*, 2019.

[23] Z. Yang, Z. Dai, Y. Yang, J. Carbonell, R. R. Salakhutdinov, and Q. V. Le, "Xlnet: Generalized autoregressive pretraining for language understanding," in *Proc. Adv. Neural Inform. Process. Syst.*, vol. 32, 2019.

[24] B. Wang and A. Komatsuzaki, "Gpt-j-6b: A 6 billion parameter autoregressive language model," 2021.

[25] S. Black, S. Biderman, E. Hallahan, Q. Anthony, L. Gao, L. Golding, H. He, C. Leahy, K. McDonell, J. Phang *et al.*, "Gpt-neox-20b: An open-source autoregressive language model," *arXiv preprint arXiv:2204.06745*, 2022.

[26] A. Q. Jiang, A. Sablayrolles, A. Mensch, C. Bamford, D. S. Chaplot, D. de las Casas, F. Bressand, G. Lengyel, G. Lample, L. Saulnier, L. R. Lavaud, M.-A. Lachaux, P. Stock, T. L. Scao, T. Lavril, T. Wang, T. Lacroix, and W. E. Sayed, "Mistral 7b," *arXiv preprint arXiv:2310.06825*, 2023.

[27] R. Li, L. B. Allal, Y. Zi, N. Muennighoff, D. Kocetkov, C. Mou, M. Marone, C. Akiki, J. Li, J. Chim, Q. Liu, E. Zheltonozhskii, T. Y. Zhuo, T. Wang, O. Dehaene, M. Davaadorj, J. Lamy-Poirier, J. Monteiro, O. Shliazhko, N. Gontier, N. Meade, A. Zebaze, M.-H. Yee, L. K. Umapathi, J. Zhu, B. Lipkin, M. Oblokulov, Z. Wang, R. Murthy, J. Stillerman, S. S. Patel, D. Abulkhanov, M. Zocca, M. Dey, Z. Zhang, N. Fahmy, U. Bhattacharyya, W. Yu, S. Singh, S. Luccioni, P. Villegas, M. Kunakov, F. Zhdanov, M. Romero, T. Lee, N. Timor, J. Ding, C. Schlesinger, H. Schoelkopf, J. Ebert, T. Dao, M. Mishra, A. Gu, J. Robinson, C. J. Anderson, B. Dolan-Gavitt, D. Contractor, S. Reddy, D. Fried, D. Bahdanau, Y. Jernite, C. M. Ferrandis, S. Hughes, T. Wolf, A. Guha, L. von Werra, and H. de Vries, "Starcoder: may the source be with you!" *Transactions on Machine Learning Research*, 2023.

[28] G. Team, T. Mesnard, C. Hardin, R. Dadashi, S. Bhupatiraju, S. Pathak, L. Sifre, M. Rivière, M. S. Kale, J. Love *et al.*, "Gemma: Open models based on gemini research and technology," *arXiv preprint arXiv:2403.08295*, 2024.

[29] L. Ouyang, J. Wu, X. Jiang, D. Almeida, C. L. Wainwright, P. Mishkin, C. Zhang, S. Agarwal, K. Slama, A. Ray, J. Schulman, J. Hilton, F. Kelton, L. Miller, M. Simens, A. Askell, P. Welinder, P. Christiano, J. Leike, and R. Lowe, "Training language models to follow instructions with human feedback," in *Proc. Adv. Neural Inform. Process. Syst.*, 2022.

[30] Z. Yao, R. Y. Aminabadi, M. Zhang, X. Wu, C. Li, and Y. He, "Zeroquant: Efficient and affordable post-training quantization for large-scale transformers," in *Proc. Adv. Neural Inform. Process. Syst.*, vol. 35, 2022, pp. 27 168–27 183.

[31] G. Xiao, J. Lin, M. Seznec, H. Wu, J. Demouth, and S. Han, "Smoothquant: Accurate and efficient post-training quantization for large language models," in *Proc. Int. Conf. Mach. Learn.*, 2023.

[32] S. Kim, C. Hooper, A. Gholami, Z. Dong, X. Li, S. Shen, M. W. Mahoney, and K. Keutzer, "Squeezellm: Dense-and-sparse quantization," in *Proc. Int. Conf. Mach. Learn.*, 2024.

[33] S. Shen, Z. Dong, J. Ye, L. Ma, Z. Yao, A. Gholami, M. W. Mahoney, and K. Keutzer, "Q-bert: Hessian based ultra low precision quantization of bert," in *Proc. AAAI Conf. Artif. Intell.*, 2020.

[34] T. Dettmers, A. Pagnoni, A. Holtzman, and L. Zettlemoyer, "Qlora: Efficient finetuning of quantized llms," in *Proc. Adv. Neural Inform. Process. Syst.*, 2023.

[35] E. Frantar, S. Ashkboos, T. Hoefler, and D. Alistarh, "Gptq: Accurate post-training quantization for generative pre-trained transformers," in *Proc. Int. Conf. Learn. Represent.*, 2023.

[36] T. Dettmers, R. Svirschevski, V. Egiazarian, D. Kuznedelev, E. Frantar, S. Ashkboos, A. Borzunov, T. Hoefler, and D. Alistarh, "Spqr: A sparse-quantized representation for near-lossless llm weight compression," in *Proc. Int. Conf. Learn. Represent.*, 2024.

[37] J. Lin, J. Tang, H. Tang, S. Yang, W.-M. Chen, W.-C. Wang, G. Xiao, X. Dang, C. Gan, and S. Han, "Awq: Activation-aware weight quantization for llm compression and acceleration," in *Proc. Mach. Learn. Syst. Conf.*, 2024.

[38] A. Fan, P. Stock, B. Graham, E. Grave, R. Gribonval, H. Jegou, and A. Joulin, "Training with quantization noise for extreme model compression," in *Proc. Int. Conf. Learn. Represent.*, 2021.

[39] H. Laurençon, L. Saulnier, L. Tronchon, S. Bekman, A. Singh, A. Lozhkov, T. Wang, S. Karamcheti, A. M. Rush, D. Kiela, M. Cord, and V. Sanh, "Obelics: An open web-scale filtered dataset of interleaved image-text documents," in *Proc. Adv. Neural Inform. Process. Syst.*, 2023.

[40] C. Schuhmann, R. Beaumont, R. Vencu, C. Gordon, R. Wightman, M. Cherti, T. Coombes, A. Katta, C. Mullis, M. Wortsman, P. Schramowski, S. Kundurthy, K. Crowson, L. Schmidt, R. Kaczmarczyk, and J. Jitsev, "Laion-5b: An open large-scale dataset for training next generation image-text models," in *Proc. Adv. Neural Inform. Process. Syst.*, 2022.

[41] K. Srinivasan, K. Raman, J. Chen, M. Bendersky, and M. Najork, "Wit: Wikipedia-based image text dataset for multimodal multilingual machine learning," in *Proc. Int. ACM SIGIR Conf. Res. Dev. Inf. Retrieval*, 2021, pp. 2443–2449.

[42] D. A. Hudson and C. D. Manning, "Gqa: A new dataset for real-world visual reasoning and compositional question answering," in *Proc. IEEE Conf. Comput. Vis. Pattern Recog.*, 2019, pp. 6700–6709.

[43] A. Singh, V. Natarajan, M. Shah, Y. Jiang, X. Chen, D. Batra, D. Parikh, and M. Rohrbach, "Towards vqa models that can read," in *Proc. IEEE Conf. Comput. Vis. Pattern Recog.*, 2019, pp. 8317–8326.

[44] P. Lu, S. Mishra, T. Xia, L. Qiu, K.-W. Chang, S.-C. Zhu, O. Tafjord, P. Clark, and A. Kalyan, "Learn to explain: Multimodal reasoning via thought chains for science question answering," in *Proc. Adv. Neural Inform. Process. Syst.*, vol. 35, 2022, pp. 2507–2521.

[45] D. Gurari, Q. Li, A. J. Stangl, A. Guo, C. Lin, K. Grauman, J. Luo, and J. P. Bigham, "Vizwiz grand challenge: Answering visual questions from blind people," in *Proc. IEEE Conf. Comput. Vis. Pattern Recog.*, 2018, pp. 3608–3617.

[46] H. Liu, C. Li, Q. Wu, and Y. J. Lee, "Visual instruction tuning," in *Proc. Adv. Neural Inform. Process. Syst.*, vol. 36, 2023, pp. 34 892–34 916.

[47] A. Awadalla, I. Gao, J. Gardner, J. Hessel, Y. Hanafy, W. Zhu, K. Marathe, Y. Bitton, S. Gadre, S. Sagawa, J. Jitsev, S. Kornblith, P. W. Koh, G. Ilharco, M. Wortsman, and L. Schmidt, "Openflamingo: An open-source framework for training large autoregressive vision-language models," 2023.

[48] Y. Liu, H. Yang, Z. Dong, K. Keutzer, L. Du, and S. Zhang, "Noisyquant: Noisy bias-enhanced post-training activation quantization for vision transformers," in *Proc. IEEE Conf. Comput. Vis. Pattern Recog.*, 2023.

[49] O. Russakovsky, J. Deng, H. Su, J. Krause, S. Satheesh, S. Ma, Z. Huang, A. Karpathy, A. Khosla, M. Bernstein *et al.*, "Imagenet large scale visual recognition challenge," *International journal of computer vision*, vol. 115, pp. 211–252, 2015.

[50] A. Krizhevsky, G. Hinton *et al.*, "Learning multiple layers of features from tiny images," *Toronto, ON, Canada*, 2009.

[51] X. Chen, H. Fang, T.-Y. Lin, R. Vedantam, S. Gupta, P. Dollár, and C. L. Zitnick, "Microsoft coco captions: Data collection and evaluation server," *arXiv preprint arXiv:1504.00325*, 2015.

[52] F. Yu, A. Seff, Y. Zhang, S. Song, T. Funkhouser, and J. Xiao, "Lsun: Construction of a large-scale image dataset using deep learning with humans in the loop," *arXiv preprint arXiv:1506.03365*, 2016.

[53] Y. Goyal, T. Khot, D. Summers-Stay, D. Batra, and D. Parikh, "Making the v in vqa matter: Elevating the role of image understanding in visual question answering," in *Proc. IEEE Conf. Comput. Vis. Pattern Recog.*, 2017, pp. 6904–6913.

[54] A. Q. Nichol and P. Dhariwal, "Improved denoising diffusion probabilistic models," in *Proc. Int. Conf. Mach. Learn.*, 2021, pp. 8162–8171.

[55] J. Ho, A. Jain, and P. Abbeel, "Denoising diffusion probabilistic models," in *Proc. Adv. Neural Inform. Process. Syst.*, vol. 33, 2020, pp. 6840–6851.

[56] K. He, X. Zhang, S. Ren, and J. Sun, "Deep residual learning for image recognition," in *Proc. IEEE Conf. Comput. Vis. Pattern Recog.*, 2016, pp. 770–778.

[57] M. Sandler, A. Howard, M. Zhu, A. Zhmoginov, and L.-C. Chen, "Mobilenetv2: Inverted residuals and linear bottlenecks," in *Proc. IEEE Conf. Comput. Vis. Pattern Recog.*, 2018, pp. 4510–4520.

[58] T. Karras, S. Laine, and T. Aila, "A style-based generator architecture for generative adversarial networks," in *Proc. IEEE Conf. Comput. Vis. Pattern Recog.*, 2019, pp. 4401–4410.

[59] J. Lin, H. Yin, W. Ping, P. Molchanov, M. Shoeybi, and S. Han, "Vila: On pre-training for visual language models," in *Proc. IEEE Conf. Comput. Vis. Pattern Recog.*, 2024, pp. 26 689–26 699.

[60] Z. Liu, Y. Lin, Y. Cao, H. Hu, Y. Wei, Z. Zhang, S. Lin, and B. Guo, "Swin transformer: Hierarchical vision transformer using shifted windows," in *Proc. IEEE Conf. Comput. Vis. Pattern Recog.*, 2021.

[61] X. Wei, R. Gong, Y. Li, X. Liu, and F. Yu, "Qdrop: Randomly dropping quantization for extremely low-bit post-training quantization," in *Proc. Int. Conf. Learn. Represent.*, 2022.

[62] Y. Shang, Z. Yuan, B. Xie, B. Wu, and Y. Yan, "Post-training quantization on diffusion models," in *Proc. IEEE Conf. Comput. Vis. Pattern Recog.*, 2023.

[63] Y. Li, S. Xu, X. Cao, X. Sun, and B. Zhang, "Q-DM: An efficient low-bit quantized diffusion model," in *Proc. Adv. Neural Inform. Process. Syst.*, 2023.

[64] I. Hubara, Y. Nahshan, Y. Hanani, R. Banner, and D. Soudry, "Accurate post training quantization with small calibration sets," in *Proc. Int. Conf. Mach. Learn.*, 2021.

[65] E. Agustsson and R. Timofte, "Ntire 2017 challenge on single image super-resolution: Dataset and study," in *Proc. IEEE Conf. Comput. Vis. Pattern Recog.*, 2017, pp. 126–135.

[66] P. Wei, Z. Xie, H. Lu, Z. Zhan, Q. Ye, W. Zuo, and L. Lin, "Component divide-and-conquer for real-world image super-resolution," in *Proc. Eur. Conf. Comput. Vis.* Springer, 2020, pp. 101–117.

[67] M. Bevilacqua, A. Roumy, C. Guillemot, and M. L. Alberi-Morel, "Low-complexity single-image super-resolution based on nonnegative neighbor embedding," in *Proc. IEEE Int. Conf. Acoust. Speech Signal Process.*, 2012.

[68] R. Zeyde, M. Elad, and M. Protter, "On single image scale-up using sparse-representations," in *Proc. Int. Conf. Curves Surfaces*, 2010, pp. 711–730.

[69] D. Martin, C. Fowlkes, D. Tal, and J. Malik, "A database of human segmented natural images and its application to evaluating segmentation algorithms and measuring ecological statistics," in *Proc. Int. Conf. Comput. Vis.*, vol. 2, 2001, pp. 416–423.

[70] J.-B. Huang, A. Singh, and N. Ahuja, "Single image super-resolution from transformed self-exemplars," in *Proc. IEEE Conf. Comput. Vis. Pattern Recog.*, 2015, pp. 5197–5206.

[71] J. Kim, J. K. Lee, and K. M. Lee, "Accurate image super-resolution using very deep convolutional networks," in *Proc. IEEE Conf. Comput. Vis. Pattern Recog.*, 2016, pp. 1646–1654.

[72] B. Lim, S. Son, H. Kim, S. Nah, and K. Mu Lee, "Enhanced deep residual networks for single image super-resolution," in *Proc. IEEE Conf. Comput. Vis. Pattern Recog.*, 2017, pp. 136–144.

[73] Y. Zhang, Y. Tian, Y. Kong, B. Zhong, and Y. Fu, "Residual dense network for image super-resolution," in *Proc. IEEE Conf. Comput. Vis. Pattern Recog.*, 2018, pp. 2472–2481.

[74] C. Ledig, L. Theis, F. Huszár, J. Caballero, A. Cunningham, A. Acosta, A. Aitken, A. Tejani, J. Totz, Z. Wang *et al.*, "Photo-realistic single image super-resolution using a generative adversarial network," in *Proc. IEEE Conf. Comput. Vis. Pattern Recog.*, 2017, pp. 4681–4690.

[75] C. Hong, H. Kim, S. Baik, J. Oh, and K. M. Lee, "Daq: Channel-wise distribution-aware quantization for deep image super-resolution networks," in *Proc. IEEE Winter Conf. Appl. Comput. Vis.*, 2022, pp. 2675–2684.

[76] Z. Yang, Y. Wang, K. Han, C. Xu, C. Xu, D. Tao, and C. Xu, "Searching for low-bit weights in quantized neural networks," in *Proc. Adv. Neural Inform. Process. Syst.*, 2020.

[77] L. Wang, X. Dong, Y. Wang, L. Liu, W. An, and Y. Guo, "Learnable lookup table for neural network quantization," in *Proc. IEEE Conf. Comput. Vis. Pattern Recog.*, 2022, pp. 12 423–12 433.

[78] L.-C. Chen, Y. Zhu, G. Papandreou, F. Schroff, and H. Adam, "Encoder-decoder with atrous separable convolution for semantic image segmentation," in *Proc. Eur. Conf. Comput. Vis.*, 2018, pp. 801–818.

[79] X. Ding, X. Zhang, N. Ma, J. Han, G. Ding, and J. Sun, "Repvgg: Making vgg-style convnets great again," in *Proc. IEEE Conf. Comput. Vis. Pattern Recog.*, 2021, pp. 13 733–13 742.

[80] M. Nagel, R. A. Amjad, M. van Baalen, C. Louizos, and T. Blankevoort, "Up or down? adaptive rounding for post-training quantization," in *Proc. Int. Conf. Mach. Learn.*, 2020.

[81] I. Radosavovic, R. P. Kosaraju, R. Girshick, K. He, and P. Dollár, "Designing network design spaces," in *Proc. IEEE Conf. Comput. Vis. Pattern Recog.*, 2020, pp. 10 428–10 436.

[82] M. Tan, B. Chen, R. Pang, V. Vasudevan, M. Sandler, A. Howard, and Q. V. Le, "Mnasnet: Platform-aware neural architecture search for mobile," in *Proc. IEEE Conf. Comput. Vis. Pattern Recog.*, 2019, pp. 2820–2828.

[83] K. Simonyan and A. Zisserman, "Very deep convolutional networks for large-scale image recognition," in *Proc. Int. Conf. Learn. Represent.*, 2015.

[84] C. Szegedy, V. Vanhoucke, S. Ioffe, J. Shlens, and Z. Wojna, "Rethinking the inception architecture for computer vision," in *Proc. IEEE Conf. Comput. Vis. Pattern Recog.*, 2016, pp. 2818–2826.

[85] Y. Li, R. Gong, X. Tan, Y. Yang, P. Hu, Q. Zhang, F. Yu, W. Wang, and S. Gu, "Brecq: Pushing the limit of post-training quantization by block reconstruction," in *Proc. Int. Conf. Learn. Represent.*, 2021.

[86] Z. Dong, Z. Yao, A. Gholami, M. W. Mahoney, and K. Keutzer, "Hawq: Hessian aware quantization of neural networks with mixed-precision," in *Proc. Int. Conf. Comput. Vis.*, 2019, pp. 293–302.

[87] M. Nagel, M. Fournarakis, Y. Bondarenko, and T. Blankevoort, "Overcoming oscillations in quantization-aware training," in *Proc. Int. Conf. Mach. Learn.*, 2022.

[88] T.-Y. Lin, P. Goyal, R. Girshick, K. He, and P. Dollár, "Focal loss for dense object detection," in *Proc. Int. Conf. Comput. Vis.*, 2017, pp. 2980–2988.

[89] Z. Yao, C. Li, X. Wu, S. Youn, and Y. He, "A comprehensive study on post-training quantization for large language models," *arXiv preprint arXiv:2303.08302*, 2023.

[90] B. Rokh, A. Azarpeyvand, and A. Khanteymoori, "A comprehensive survey on model quantization for deep neural networks in image classification," *ACM Trans. Intell. Syst. Technol.*, vol. 14, no. 6, pp. 1–50, 2023.

[91] A. Gholami, S. Kim, Z. Dong, Z. Yao, M. W. Mahoney, and K. Keutzer, "A survey of quantization methods for efficient neural network inference," in *Low-power computer vision*. Chapman and Hall/CRC, 2022, pp. 291–326.

[92] S. Li, X. Ning, L. Wang, T. Liu, X. Shi, S. Yan, G. Dai, H. Yang, and Y. Wang, "Evaluating quantized large language models," *arXiv preprint arXiv:2402.18158*, 2024.

[93] K. Egashira, M. Vero, R. Staab, J. He, and M. Vechev, "Exploiting llm quantization," *arXiv preprint arXiv:2405.18137*, 2024.

[94] Z. Yao, X. Wu, C. Li, S. Youn, and Y. He, "Exploring post-training quantization in llms from comprehensive study to low rank compensation," in *Proc. AAAI Conf. Artif. Intell.*, vol. 38, no. 17, 2024, pp. 19 377–19 385.

[95] A. Shen, Z. Lai, and D. Li, "Exploring quantization techniques for large-scale language models: Methods, challenges and future directions," in *Proc. Int. Conf. Cyber Secur. Inf. Eng.*, 2024, pp. 783–790.

[96] T. Dettmers and L. Zettlemoyer, "The case for 4-bit precision: k-bit inference scaling laws," in *Proc. Int. Conf. Mach. Learn.* PMLR, 2023, pp. 7750–7774.

[97] T. Chen, B. Ji, T. Ding, B. Fang, G. Wang, Z. Zhu, L. Liang, Y. Shi, S. Yi, and X. Tu, "Only train once: A one-shot neural network training and pruning framework," in *Proc. Adv. Neural Inform. Process. Syst.*, 2021.

[98] H. Yang, W. Wen, and H. Li, "Deephoyer: Learning sparser neural network with differentiable scale-invariant sparsity measures," in *Proc. Int. Conf. Learn. Represent.*, 2020.

[99] S. Lin, R. Ji, Y. Li, C. Deng, and X. Li, "Towards compact convnets via structure-sparsity regularized filter pruning," *arXiv preprint arXiv:1901.07827*, 2019.

[100] Y. Zhou, Y. Zhang, Y. Wang, and Q. Tian, "Accelerate cnn via recursive bayesian pruning," in *Proc. Int. Conf. Comput. Vis.*, 2019, pp. 3306–3315.

[101] M. van Baalen, C. Louizos, M. Nagel, R. A. Amjad, Y. Wang, T. Blankevoort, and M. Welling, "Bayesian bits: Unifying quantization and pruning," in *Proc. Adv. Neural Inform. Process. Syst.*, 2020.

[102] T. Chen, L. Liang, T. Ding, Z. Zhu, and I. Zharkov, "Otov2: Automatic, generic, user-friendly," in *Proc. Int. Conf. Learn. Represent.*, 2023.

[103] B. Li, B. Wu, J. Su, G. Wang, and L. Lin, "Eagleeye: Fast sub-net evaluation for efficient neural network pruning," in *Proc. Eur. Conf. Comput. Vis.*, 2020.

[104] S. Zhong, Z. You, J. Zhang, S. Zhao, Z. LeClaire, Z. Liu, D. Zha, V. Chaudhary, S. Xu, and X. Hu, "One less reason for filter pruning: Gaining free adversarial robustness with structured grouped kernel pruning," in *Proc. Adv. Neural Inform. Process. Syst.*, 2023.

[105] J. Chen, S. Chen, and S. J. Pan, "Storage efficient and dynamic flexible runtime channel pruning via deep reinforcement learning," in *Proc. Int. Conf. Learn. Represent.*, vol. 33, 2020, pp. 14 747–14 758.

[106] J. Frankle, G. K. Dziugaite, D. M. Roy, and M. Carbin, "Linear mode connectivity and the lottery ticket hypothesis," in *Proc. Int. Conf. Mach. Learn.*, 2020.

[107] Z. Tao, Z. Zhang, Y. Huang, X. Zeng, K. Shuang, and X. Li, "Neuron-level structured pruning using polarization regularizer," in *Proc. Adv. Neural Inform. Process. Syst.*, 2020.

[108] H. Li, A. Kadav, I. Durdanovic, H. Samet, and H. P. Graf, "Pruning filters for efficient convnets," in *Proc. Int. Conf. Learn. Represent.*, 2017.

[109] S. Han, J. Pool, J. Tran, and W. J. Dally, "Learning both weights and connections for efficient neural networks," in *Proc. Adv. Neural Inform. Process. Syst.*, vol. 28, 2015.

[110] G. Hinton, O. Vinyals, and J. Dean, "Distilling the knowledge in a neural network," in *Proc. Adv. Neural Inform. Process. Syst.*, 2014.

[111] K. Yu, C. Yu, T. Zhang, X. Zhao, S. Yang, H. Wang, Q. Zhang, and Q. Xu, "Temporal separation with entropy regularization for knowledge distillation in spiking neural networks," in *Proc. IEEE Conf. Comput. Vis. Pattern Recog.*, 2025.

[112] Q. Xiang, M. Zhang, Y. Shang, J. Wu, Y. Yan, and L. Nie, "Dkdm: Data-free knowledge distillation for diffusion models with any architecture," in *Proc. IEEE Conf. Comput. Vis. Pattern Recog.*, 2025.

[113] J. Lee, D. Das, M. Hayat, S. Choi, K. Hwang, and F. Porikli, "Customkd: Customizing large vision foundation for edge model improvement via knowledge distillation," in *Proc. IEEE Conf. Comput. Vis. Pattern Recog.*, 2025.

[114] H. Lin, X. Cheng, X. Wu, F. Yang, D. Shen, Z. Wang, Q. Song, and W. Yuan, "Cat: Cross attention in vision transformer," *Proc. IEEE Int. Conf. Multimedia Expo*, 2021.

[115] Z. Xia, X. Pan, S. Song, L. E. Li, and G. Huang, "Vision transformer with deformable attention," in *Proc. IEEE Conf. Comput. Vis. Pattern Recog.*, 2022.
